# Supplementary material for: High-Fidelity Qutrit Entangling Gates for Superconducting Circuits
Source: arXiv:2206.07216 source file (2023-06-30)
Supplement: Supplementary file 2 [file supp_preamble.tex]

\usepackage{amsthm}
\usepackage{mathtools}
\usepackage{physics}
\usepackage{xcolor}
\usepackage{graphicx}
\usepackage[left=23mm,right=13mm,top=35mm,columnsep=15pt]{geometry} 
\usepackage{adjustbox}
\usepackage{placeins}
\usepackage[T1]{fontenc}
\usepackage{lipsum}
\usepackage{csquotes}
\usepackage{xcolor}


% \usepackage[pdftex, pdftitle={Article}, pdfauthor={Author}]{hyperref} % 

% \hypersetup{
%     colorlinks=true,
%     linkcolor=red,
%     filecolor=magenta,      
%     urlcolor=cyan,
% }
\usepackage{xcolor}
\usepackage{cleveref} % smart reference
\newcommand{\alexis}[1]{{\textsf{{\color{red}{Alexis' comment:}   #1 }}}}

% Tikz
\usepackage{tikz}

\renewcommand{\a}{{\alpha}}



\usepackage[normalem]{ulem} % For \sout

% Joel's macros
\newcommand{\mc}{\mathcal}
\newcommand{\bb}{\mathbb}
\newcommand{\cn}{{\textcolor{blue}{[citation needed]}}}

\newcommand{\dbra}[1]{\ensuremath{\langle\!\langle #1|}}
\newcommand{\dket}[1]{\ensuremath{|#1\rangle\!\rangle}}

%from https://stackoverflow.com/a/1812477/3183467
\makeatletter
\def\dketbra#1{\def\tempa{#1}\futurelet\next\dketbra@i}% Save first argument
\def\dketbra@i{\ifx\next\bgroup\expandafter\dketbra@ii\else\expandafter\dketbra@end\fi}%Check brace
\def\dketbra@ii#1{| \tempa \rangle\!\rangle\!\langle\!\langle #1 |}%Two args
\def\dketbra@end{| \tempa \rangle\!\rangle\!\langle\!\langle \tempa |}%Single args
\makeatother

\makeatletter
\def\dbraket#1{\def\tempa{#1}\futurelet\next\dbraket@i}% Save first argument
\def\dbraket@i{\ifx\next\bgroup\expandafter\dbraket@ii\else\expandafter\dbraket@end\fi}%Check brace
\def\dbraket@ii#1{\langle\!\langle \tempa | #1 \rangle\!\rangle}%Two args
\def\dbraket@end{\langle\!\langle \tempa | \tempa \rangle\!\rangle}%Single args
\makeatother
